# Supplementary material for: Goodness of fit of logistic models for random graphs
Source: arXiv:1508.00286 ancillary file (2017-01-06)
Supplement: Supplementary file 1 [file appendix.pdf]

# Supplementary files of “Goodness of fit of logistic models for random graphs” : Appendix

Pierre Latouche

Laboratoire SAMM, EA 4543, Université Paris 1 Panthéon-Sorbonne, France  
and

Stéphane Robin

AgroParisTech, UMR 518, MIA, Paris, France

INRA, UMR 518, MIA, Paris, France

and

Sarah Ouadah

AgroParisTech, UMR 518, MIA, Paris, France

INRA, UMR 518, MIA, Paris, France

November 23, 2015

# A Appendix

## A.1 Proof of Proposition 1

Let us start by showing that:

$$\log p(Y|Z, \alpha, \beta) \geq \log \sqrt{h(Z, \alpha, \beta, \xi)},$$

where  $\xi$  is an  $n \times n$  positive real matrix. We use the bound on the log-logistic function introduced by [1] from Taylor expansions:

$$\log g(x) \geq \log g(\xi) + \frac{x - \xi}{2} - \lambda(\xi)(x^2 - \xi^2), \forall (x, \xi) \in \mathbb{R} \times \mathbb{R}^+, \quad (1)$$

where  $\lambda(\xi) = (g(\xi) - 1/2)/(2\xi)$ . Note that (1) is an even function and therefore we can consider only positive values of  $x$  without loss of generality. Since

$$\log p(Y_{ij}|Z_i, Z_j, \alpha, \beta) = Y_{ij}(Z_i^\top \alpha Z_j + x_{ij}^\top \beta) + \log g(-Z_i^\top \alpha Z_j - x_{ij}^\top \beta),$$

then

$$\begin{aligned} \log p(Y_{ij}|Z_i, Z_j, \alpha, \beta) &\geq Y_{ij}(Z_i^\top \alpha Z_j + x_{ij}^\top \beta) + \log g(\xi_{ij}) - \frac{Z_i^\top \alpha Z_j + x_{ij}^\top \beta + \xi_{ij}}{2} \\ &\quad - \lambda(\xi_{ij})((Z_i^\top \alpha Z_j + x_{ij}^\top \beta)^2 - \xi_{ij}^2) \\ &= (Y_{ij} - \frac{1}{2})(Z_i^\top \alpha Z_j + x_{ij}^\top \beta) - \frac{\xi_{ij}}{2} + \log g(\xi_{ij}) \\ &\quad - \lambda(\xi_{ij})((Z_i^\top \alpha Z_j + x_{ij}^\top \beta)^2 - \xi_{ij}^2). \end{aligned}$$

Note that for undirected networks, the matrix  $\xi$  has to be symmetric, *i.e.*  $\xi_{ij} = \xi_{ji}, \forall i \neq j$ .

We then have

$$\log p(Y|Z, \alpha, \beta) = \frac{1}{2} \sum_{i \neq j}^n \log p(Y_{ij}|Z_i, Z_j, \alpha, \beta).$$

Therefore

$$\log p(Y|Z, \alpha, \beta) \geq \log \sqrt{h(Z, \alpha, \beta, \xi)}.$$

Finally,

$$\begin{aligned}
\mathcal{L}_K(q) &= \sum_Z \int q(Z, \pi, \alpha, \beta, \gamma, \eta) \log \frac{p(Y, Z, \pi, \alpha, \beta, \gamma, \eta)}{q(Z, \pi, \alpha, \beta, \gamma, \eta)} d\pi d\alpha d\beta d\gamma d\eta \\
&= \sum_Z \int q(Z, \pi, \alpha, \beta, \gamma, \eta) \log \frac{p(Y|Z, \alpha, \beta) p(Z, \pi, \alpha, \beta, \gamma, \eta)}{q(Z, \pi, \alpha, \beta, \gamma, \eta)} d\pi d\alpha d\beta d\gamma d\eta \\
&\geq \sum_Z \int q(Z, \pi, \alpha, \beta, \gamma, \eta) \log \frac{\sqrt{h(Z, \alpha, \beta, \xi)} p(Z, \pi, \alpha, \beta, \gamma, \eta)}{q(Z, \pi, \alpha, \beta, \gamma, \eta)} d\pi d\alpha d\beta d\gamma d\eta \\
&= \mathcal{L}_K(q; \xi).
\end{aligned}$$

## A.2 Proof of Proposition 2

$$\begin{aligned}
\log q(Z_i) &= \mathbb{E}_{Z \setminus i, \alpha, \beta, \pi} \left[ \frac{1}{2} \log h(Z, \alpha, \beta, \xi) + \log p(Z|\pi) \right] + \text{cst} \\
&= \mathbb{E}_{Z \setminus i, \alpha, \beta, \pi} \left[ \frac{1}{2} \sum_{i \neq j}^n \left\{ (Y_{ij} - \frac{1}{2}) Z_i^\top \alpha Z_j - \lambda(\xi_{ij}) ((Z_i^\top \alpha Z_j)^2 + 2Z_i^\top \alpha Z_i x_{ij}^\top \beta) \right\} \right. \\
&\quad \left. + \sum_{k=1}^n Z_{ik} \log \pi_k \right] + \text{cst}.
\end{aligned}$$

Note that

$$\begin{aligned}
\mathbb{E}_{Z_j, \alpha} [Z_i^\top \alpha Z_j] &= \mathbb{E}_{Z_j, \alpha} \left[ \sum_{k,l} Z_{ik} \alpha_{kl} Z_{jl} \right] \\
&= \sum_{k=1}^K Z_{ik} \left\{ \sum_{l=1}^K (m_\alpha)_{kl} \tau_{jl} \right\}.
\end{aligned}$$

Furthermore

$$\begin{aligned}
\mathbb{E}_{Z_j, \alpha} [(Z_i^\top \alpha Z_j)^2] &= \mathbb{E}_{Z_j, \alpha} \left[ \left( \sum_{k,l} Z_{ik} \alpha_{kl} Z_{jl} \right)^2 \right] \\
&= \mathbb{E}_{Z_j, \alpha} \left[ \sum_{k,k',l,l'} Z_{ik} Z_{ik'} \alpha_{kl} \alpha_{k'l'} Z_{jl} Z_{jl'} \right].
\end{aligned} \tag{2}$$

Because all vectors  $Z_i$  are sampled from a multinomial distribution with parameters  $(1, \pi)$ , all terms  $Z_{ik} Z_{ik'} = 0$  for  $k \neq k'$  and  $Z_{ik}^2 = Z_{ik}$  in (2). Therefore

$$(Z_i^\top \alpha Z_j)^2 = \sum_{k,l} Z_{ik} \alpha_{kl}^2 Z_{jl}. \tag{3}$$

This leads to

$$\mathbb{E}_{Z_j, \alpha} [(Z_i^\top \alpha Z_j)^2] = \sum_{k=1}^K Z_{ik} \left\{ \sum_{l=1}^K \mathbb{E}_{\alpha_{kl}} [\alpha_{kl}^2] \tau_{jl} \right\}.$$

Finally

$$\begin{aligned} \log q(Z_i) = & \sum_{k=1}^K Z_{ik} \left\{ \sum_{l=1}^K (m_\alpha)_{kl} \frac{1}{2} \sum_{j \neq i}^n \left( (Y_{ij} - \frac{1}{2}) - 2\lambda(\xi_{ij}) x_{ij}^\top m_\beta \right) \tau_{jl} - \sum_{l=1}^K \mathbb{E}_{\alpha_{kl}}[\alpha_{kl}^2] \frac{1}{2} \sum_{j \neq i}^n \lambda(\xi_{ij}) \tau_{jl} \right. \\ & + \sum_{l=1}^K (m_\alpha)_{lk} \frac{1}{2} \sum_{j \neq i}^n \left( (Y_{ji} - \frac{1}{2}) - 2\lambda(\xi_{ji}) x_{ji}^\top m_\beta \right) \tau_{jl} - \sum_{l=1}^K \mathbb{E}_{\alpha_{lk}}[\alpha_{lk}^2] \frac{1}{2} \sum_{j \neq i}^n \lambda(\xi_{ji}) \tau_{jl} \\ & \left. + \psi(e_k^n) - \psi\left(\sum_{l=1}^K e_l^n\right) \right\} + \text{cst.} \end{aligned}$$

Since  $(m_\alpha)_{kl} = (m_\alpha)_{lk}$ ,  $\mathbb{E}_{\alpha_{kl}}[\alpha_{kl}^2] = \mathbb{E}_{\alpha_{lk}}[\alpha_{lk}^2]$ ,  $Y_{ij} = Y_{ji}$ ,  $x_{ij} = x_{ji}$ ,  $\xi_{ij} = \xi_{ji}$ , then

$$\begin{aligned} \log q(Z_i) = & \sum_{k=1}^K Z_{ik} \left\{ \sum_{l=1}^K (m_\alpha)_{kl} \sum_{j \neq i}^n \left( (Y_{ij} - \frac{1}{2}) - 2\lambda(\xi_{ij}) x_{ij}^\top m_\beta \right) \tau_{jl} - \sum_{l=1}^K \mathbb{E}_{\alpha_{kl}}[\alpha_{kl}^2] \sum_{j \neq i}^n \lambda(\xi_{ij}) \tau_{jl} \right. \\ & \left. + \psi(e_k^n) - \psi\left(\sum_{l=1}^K e_l^n\right) \right\} + \text{cst.} \end{aligned}$$

Therefore

$$q(Z_i) = \mathcal{M}(Z_i; 1, \tau_i),$$

where  $\sum_{k=1}^K \tau_{ik} = 1$  and

$$\begin{aligned} \tau_{ik} \propto \exp \left\{ \sum_{l=1}^K (m_\alpha)_{kl} \sum_{j \neq i}^n \left( (Y_{ij} - \frac{1}{2}) - 2\lambda(\xi_{ij}) x_{ij}^\top m_\beta \right) \tau_{jl} - \sum_{l=1}^K \mathbb{E}_{\alpha_{kl}}[\alpha_{kl}^2] \sum_{j \neq i}^n \lambda(\xi_{ij}) \tau_{jl} \right. \\ \left. + \psi(e_k^n) - \psi\left(\sum_{l=1}^K e_l^n\right) \right\}. \end{aligned}$$

### A.3 Proof of Proposition 3

$$\begin{aligned} \log q(\pi) &= \mathbb{E}_Z [\log p(Z|\pi) + \log p(\pi)] + \text{cst} \\ &= \sum_{i=1}^n \sum_{k=1}^K \tau_{ik} \log \pi_k + \sum_{k=1}^K (e_0 - 1) \log \pi_k + \text{cst} \\ &= \sum_{k=1}^K \left( e_0 + \sum_{i=1}^n \tau_{ik} - 1 \right) \log \pi_k + \text{cst}. \end{aligned}$$

Therefore

$$q(\pi) = \text{Dir}(\pi; e^n),$$

where  $e_k^n = e_0 + \sum_{i=1}^n \tau_{ik}$ ,  $\forall k \in \{1, \dots, K\}$ .

#### A.4 Proof of Proposition 4

$$\begin{aligned}
\log q(\beta) &= \mathbb{E}_{Z, \alpha, \eta} \left[ \frac{1}{2} \log h(Z, \alpha, \beta, \xi) + \log p(\beta|\eta) \right] + \text{cst} \\
&= \mathbb{E}_{Z, \alpha, \eta} \left[ \frac{1}{2} \sum_{i \neq j}^n \left\{ (Y_{ij} - 1/2) x_{ij}^\top \beta - \lambda(\xi_{ij}) \left( (x_{ij}^\top \beta)^2 + 2Z_i^\top \alpha Z_j x_{ij}^\top \beta \right) \right\} - \frac{\eta}{2} \beta^\top \beta \right] + \text{cst} \\
&= \beta^\top \left\{ \frac{1}{2} \sum_{i \neq j}^n \left( Y_{ij} - \frac{1}{2} - 2\lambda(\xi_{ij}) \tau_i^\top m_\alpha \tau_j \right) x_{ij} \right\} - \frac{1}{2} \beta^\top \left\{ \frac{c_n}{d_n} I_d + \sum_{i \neq j}^n \lambda(\xi_{ij}) x_{ij} x_{ij}^\top \right\} \beta + \text{cst}.
\end{aligned}$$

Therefore

$$q(\beta) = \mathcal{N}(\beta; m_\beta, S_\beta),$$

where

$$S_\beta^{-1} = \frac{c_n}{d_n} I_d + \sum_{i \neq j}^n \lambda(\xi_{ij}) x_{ij} x_{ij}^\top,$$

and

$$m_\beta = S_\beta \frac{1}{2} \sum_{i \neq j}^n \left( Y_{ij} - \frac{1}{2} - 2\lambda(\xi_{ij}) \tau_i^\top m_\alpha \tau_j \right) x_{ij}.$$

#### A.5 Proof of Proposition 5

$$\begin{aligned}
\log q(\gamma) &= \mathbb{E}_\alpha [\log p(\alpha|\gamma) + \log p(\gamma)] + \text{cst} \\
&= \mathbb{E}_\alpha \left[ \sum_{k \leq l}^K \frac{1}{2} \log(\gamma) - \sum_{k \leq l}^K \frac{\gamma}{2} \alpha_{kl}^2 \right] + (a_0 - 1) \log \gamma - b_0 \gamma + \text{cst} \\
&= (a_0 + \frac{K(K+1)}{4} - 1) \log \gamma - \left( b_0 + \frac{1}{2} \sum_{k \leq l}^K \mathbb{E}_{\alpha_{kl}} [\alpha_{kl}^2] \right) \gamma + \text{cst}.
\end{aligned}$$

Therefore

$$q(\gamma) = \text{Gam}(\gamma; a_n, b_n),$$

where  $a_n = a_0 + \frac{K(K+1)}{4}$  and  $b_n = b_0 + \frac{1}{2} \sum_{k \leq l}^K \mathbb{E}_{\alpha_{kl}} [\alpha_{kl}^2]$ .

#### A.6 Proof of Proposition 6

$$\begin{aligned}
\log q(\eta) &= \mathbb{E}_\beta [\log p(\beta|\eta) + \log p(\eta)] + \text{cst} \\
&= \mathbb{E}_\beta \left[ \frac{d}{2} \log \eta - \frac{\eta}{2} \beta^\top \beta \right] + (c_0 - 1) \log \eta - d_0 \eta + \text{cst} \\
&= (c_0 + \frac{d}{2} - 1) \log \eta - (d_0 + \frac{1}{2} \text{Tr}(S_\beta) + \frac{1}{2} m_\beta^\top m_\beta) \eta + \text{cst}.
\end{aligned}$$

Therefore

$$q(\eta) = \text{Gam}(\eta; c_n, d_n),$$

where  $c_n = c_0 + \frac{d}{2}$  and  $d_n = d_0 + \frac{1}{2}\text{Tr}(S_\beta) + \frac{1}{2}m_\beta^\top m_\beta$ .

## A.7 Proof of Proposition 7

$$\begin{aligned} \log q(\alpha) &= \mathbb{E}_{Z, \beta, \gamma} \left[ \frac{1}{2} \log h(Z, \alpha, \beta, \xi) + \log p(\alpha | \gamma) \right] + \text{cst} \\ &= \mathbb{E}_{Z, \beta, \gamma} \left[ \frac{1}{2} \sum_{i \neq j}^n \left\{ (Y_{ij} - \frac{1}{2}) Z_i^\top \alpha Z_j - \lambda(\xi_{ij}) \left( (Z_i^\top \alpha Z_j)^2 + 2 Z_i^\top \alpha Z_j x_{ij}^\top \beta \right) \right\} \right. \\ &\quad \left. - \sum_{k \leq l}^K \frac{\gamma}{2} \alpha_{kl}^2 \right] + \text{cst}. \end{aligned} \quad (4)$$

We have  $Z_i^\top \alpha Z_j = \sum_{k,l}^K Z_{ik} \alpha_{kl} Z_{jl}$  and  $(Z_i^\top \alpha Z_j)^2 = \sum_{k,l}^K Z_{ik} \alpha_{kl}^2 Z_{jl} = Z_i^\top A Z_j$  (see Eq. 3) with  $A$  the  $K \times K$  matrix such that  $A_{kl} = \alpha_{kl}^2$ . Moreover, any expression of the form  $(1/2) \sum_{i \neq j}^n c_{ij} Z_i^\top B Z_j$  where  $B$  is a symmetric  $K \times K$  matrix and  $c_{ij} = c_{ji}$  can be written

$$\begin{aligned} \frac{1}{2} \sum_{i \neq j}^n c_{ij} Z_i^\top B Z_j &= \frac{1}{2} \sum_{i \neq j}^n c_{ij} \sum_{k,l}^K Z_{ik} B_{kl} Z_{jl} \\ &= \frac{1}{2} \sum_{i \neq j}^n c_{ij} \left( \sum_{k=1}^K Z_{ik} B_{kk} Z_{jk} + \sum_{k < l}^K Z_{ik} B_{kl} Z_{jl} + \sum_{k < l}^K Z_{jk} B_{lk} Z_{il} \right) \\ &= \sum_{k=1}^K B_{kk} \frac{1}{2} \sum_{i \neq j}^n c_{ij} Z_{ik} Z_{jk} + \sum_{k < l}^K B_{kl} \left( \frac{1}{2} \sum_{i \neq j}^n c_{ij} Z_{ik} Z_{jl} + \frac{1}{2} \sum_{i \neq j}^n c_{ij} Z_{jk} Z_{il} \right). \end{aligned}$$

By exchanging the role of  $i$  and  $j$  in the sum of the last term and since  $c_{ij} = c_{ji}$ , we obtain

$$\frac{1}{2} \sum_{i \neq j}^n c_{ij} Z_i^\top B Z_j = \sum_{k=1}^K B_{kk} \frac{1}{2} \sum_{i \neq j}^n c_{ij} Z_{ik} Z_{jk} + \sum_{k < l}^K B_{kl} \sum_{i \neq j}^n c_{ij} Z_{ik} Z_{jl}. \quad (5)$$

Using (5) in (4) leads to

$$\begin{aligned}
\log q(\alpha) = & \sum_{k=1}^K \alpha_{kk} \sum_{i \neq j}^n \left( \frac{1}{2} (Y_{ij} - \frac{1}{2}) - \lambda(\xi_{ij}) x_{ij}^\top m_\beta \right) \tau_{ik} \tau_{jk} \\
& + \sum_{k < l}^K \alpha_{kl} \sum_{i \neq j}^n \left( (Y_{ij} - \frac{1}{2}) - 2\lambda(\xi_{ij}) x_{ij}^\top m_\beta \right) \tau_{ik} \tau_{jl} \\
& - \sum_{k=1}^K \alpha_{kk}^2 \sum_{i \neq j}^n \frac{1}{2} \lambda(\xi_{ij}) \tau_{ik} \tau_{jk} - \sum_{k < l}^K \alpha_{kl}^2 \sum_{i \neq j}^n \lambda(\xi_{ij}) \tau_{ik} \tau_{jl} \\
& - \sum_{k \leq l}^K \frac{a_n}{2b_n} \alpha_{kl}^2.
\end{aligned}$$

Therefore

$$q(\alpha) = \prod_{k \neq l}^K \mathcal{N}(\alpha_{kl}; (m_\alpha)_{kl}, (\sigma_\alpha^2)_{kl}),$$

where

$$\begin{aligned}
(\sigma_\alpha^2)_{kk}^{-1} &= \frac{a_n}{b_n} + \sum_{i \neq j}^n \lambda(\xi_{ij}) \tau_{ik} \tau_{jk}, \forall k, \\
(\sigma_\alpha^2)_{kl}^{-1} &= \frac{a_n}{b_n} + 2 \sum_{i \neq j}^n \lambda(\xi_{ij}) \tau_{ik} \tau_{jl}, \forall k \neq l, \\
(m_\alpha)_{kk} &= (\sigma_\alpha^2)_{kk} \sum_{i \neq j}^n \left( \frac{1}{2} (Y_{ij} - \frac{1}{2}) - \lambda(\xi_{ij}) x_{ij}^\top m_\beta \right) \tau_{ik} \tau_{jk} \\
(m_\alpha)_{kl} &= (\sigma_\alpha^2)_{kl} \sum_{i \neq j}^n \left( (Y_{ij} - \frac{1}{2}) - 2\lambda(\xi_{ij}) x_{ij}^\top m_\beta \right) \tau_{ik} \tau_{jl}.
\end{aligned}$$

## A.8 Proof of Proposition 8

Keeping only the terms that do depend on  $\xi_{ij}$  in (7), the lower bound is given by

$$\begin{aligned}
\mathcal{L}_K(q; \xi) &= \frac{1}{2} \sum_{i \neq j}^n \left\{ \log g(\xi_{ij}) - \frac{\xi_{ij}}{2} - \lambda(\xi_{ij}) \left( \mathbb{E}_{Z_i, Z_j, \alpha} [(Z_i^\top \alpha Z_j)^2] + 2 \mathbb{E}_{Z_i, Z_j, \alpha} [Z_i^\top \alpha Z_j] x_{ij}^\top \mathbb{E}_\beta [\beta] \right. \right. \\
&\quad \left. \left. + \mathbb{E}_\beta [(x_{ij}^\top \beta)^2] - \xi_{ij}^2 \right) \right\} + \text{cst} \\
&= \frac{1}{2} \sum_{i \neq j}^n \left\{ \log g(\xi_{ij}) - \frac{\xi_{ij}}{2} - \lambda(\xi_{ij}) \left( \sum_{k, l}^K \tau_{ik} \tau_{jl} \mathbb{E}_{\alpha_{kl}} [\alpha_{kl}^2] + 2 \sum_{k, l}^K \tau_{ik} \tau_{jl} (m_\alpha)_{kl} x_{ij}^\top m_\beta \right. \right. \\
&\quad \left. \left. + \text{Tr}(x_{ij} x_{ij}^\top (S_\beta + m_\beta m_\beta^\top)) - \xi_{ij}^2 \right) \right\} + \text{cst}.
\end{aligned}$$

The partial derivative of the lower bound with respect to  $\xi_{ij}$  is

$$\begin{aligned} \frac{\partial \mathcal{L}_K}{\partial \xi_{ij}}(q; \xi) = & g(-\xi_{ij}) - \frac{1}{2} - \lambda'(\xi_{ij}) \left( \sum_{k,l}^K \tau_{ik} \tau_{jl} \mathbb{E}_{\alpha_{kl}}[\alpha_{kl}^2] + 2 \sum_{k,l}^K \tau_{ik} \tau_{jl} (m_\alpha)_{kl} x_{ij}^\top m_\beta \right. \\ & \left. + \text{Tr}(x_{ij} x_{ij}^\top (S_\beta + m_\beta m_\beta^\top)) - \xi_{ij}^2 \right) + 2\lambda(\xi_{ij}) \xi_{ij}, \end{aligned}$$

and

$$\begin{aligned} \frac{\partial \mathcal{L}_K}{\partial \xi_{ij}}(q; \xi) = & -\lambda'(\xi_{ij}) \left( \sum_{k,l}^K \tau_{ik} \tau_{jl} \mathbb{E}_{\alpha_{kl}}[\alpha_{kl}^2] + 2 \sum_{k,l}^K \tau_{ik} \tau_{jl} (m_\alpha)_{kl} x_{ij}^\top m_\beta \right. \\ & \left. + \text{Tr}(x_{ij} x_{ij}^\top (S_\beta + m_\beta m_\beta^\top)) - \xi_{ij}^2 \right). \quad (6) \end{aligned}$$

Finally,  $\lambda(\xi_{ij})$  is a strictly decreasing function for positive values of  $\xi_{ij}$ . Thus,  $\lambda'(\xi_{ij}) \neq 0$  and therefore if we set (6) to zero, we obtain

$$\xi_{ij}^2 = \sum_{k,l}^K \tau_{ik} \tau_{jl} \mathbb{E}_{\alpha_{kl}}[\alpha_{kl}^2] + 2 \sum_{k,l}^K \tau_{ik} \tau_{jl} (m_\alpha)_{kl} x_{ij}^\top m_\beta + \text{Tr}(x_{ij} x_{ij}^\top (S_\beta + m_\beta m_\beta^\top)).$$

Note that  $\xi_{ij} = \xi_{ji}$ .

## A.9 Proof of Proposition 9

$$\mathcal{L}_K(q; \xi) = \mathbb{E}_{Z, \pi, \alpha, \beta, \gamma, \eta} \left[ \log \sqrt{h(Z, \alpha, \beta, \xi)} + \log p(Z, \pi, \alpha, \beta, \gamma, \eta) \right] - \mathbb{E}_{Z, \pi, \alpha, \beta, \gamma, \eta} [\log q(Z, \pi, \alpha, \beta, \gamma, \eta)]$$

$$\begin{aligned}
\mathcal{L}_K(q; \xi) = & \frac{1}{2} \sum_{i \neq j}^n \left\{ (Y_{ij} - \frac{1}{2})(\mathbb{E}_{Z_i, Z_j, \alpha}[Z_i^\top \alpha Z_j] + x_{ij}^\top \mathbb{E}_\beta[\beta]) + \log g(\xi_{ij}) - \frac{\xi_{ij}}{2} \right. \\
& \left. - \lambda(\xi_{ij}) \left( \mathbb{E}_{Z_i, Z_j, \alpha}[(Z_i^\top \alpha Z_j)^2] + 2\mathbb{E}_{Z_i, Z_j, \alpha}[Z_i^\top \alpha Z_j] x_{ij}^\top \mathbb{E}_\beta[\beta] + \mathbb{E}_\beta[(x_{ij}^\top \beta)^2] - \xi_{ij}^2 \right) \right\} \\
& + \sum_{i=1}^n \sum_{k=1}^K \mathbb{E}_{Z_i}[Z_{ik}] \mathbb{E}_\pi[\log \pi_k] - \log C(e) + \sum_{k=1}^K (e_0 - 1) \mathbb{E}_\pi[\log \pi_k] - \frac{K(K+1)}{4} \log(2\pi) \\
& + \frac{K(K+1)}{4} \mathbb{E}_\gamma[\log \gamma] - \frac{\mathbb{E}_\gamma[\gamma]}{2} \sum_{k \leq l}^K \mathbb{E}_{\alpha_{kl}}[\alpha_{kl}^2] - \frac{d}{2} \log(2\pi) + \frac{d}{2} \mathbb{E}_\eta[\log \eta] - \frac{\mathbb{E}_\eta[\eta]}{2} \mathbb{E}_\beta[\beta^\top \beta] \\
& - \log \Gamma(a_0) + a_0 \log b_0 + (a_0 - 1) \mathbb{E}_\gamma[\log \gamma] - b_0 \mathbb{E}_\gamma[\gamma] - \log \Gamma(c_0) \\
& + c_0 \log d_0 + (c_0 - 1) \mathbb{E}_\eta[\log \eta] - d_0 \mathbb{E}_\eta[\eta] - \sum_{i=1}^n \sum_{k=1}^K \mathbb{E}_{Z_i}[Z_{ik}] \log \tau_{ik} + \log C(e^n) \\
& - \sum_{k=1}^K (e_k^n - 1) \mathbb{E}_\pi[\log \pi_k] + \frac{K(K+1)}{4} \log(2\pi) + \frac{1}{2} \sum_{k \leq l}^K \log(\sigma_\alpha^2)_{kl} + \frac{1}{2} \sum_{k \leq l}^K (\sigma_\alpha^2)_{kl}^{-1} \mathbb{E}_{\alpha_{kl}}[\alpha_{kl}^2] \\
& - \sum_{k \leq l}^K (\sigma_\alpha^2)_{kl}^{-1} \mathbb{E}_{\alpha_{kl}}[\alpha_{kl}] (m_\alpha)_{kl} + \frac{1}{2} \sum_{k \leq l}^K (\sigma_\alpha^2)_{kl}^{-1} (m_\alpha)_{kl}^2 + \frac{d}{2} \log(2\pi) + \frac{1}{2} \log |S_\beta| \\
& + \frac{1}{2} \mathbb{E}_\beta[\beta^\top S_\beta^{-1} \beta] - \mathbb{E}_\beta[\beta]^\top S_\beta^{-1} m_\beta + \frac{1}{2} m_\beta^\top S_\beta^{-1} m_\beta + \log \Gamma(a_n) - a_n \log b_n \\
& - (a_n - 1) \mathbb{E}_\gamma[\log \gamma] + b_n \mathbb{E}_\gamma[\gamma] + \log \Gamma(c_n) - c_n \log d_n - (c_n - 1) \mathbb{E}_\eta[\log \eta] \\
& + d_n \mathbb{E}_\eta[\eta], \quad (7)
\end{aligned}$$

where  $C(x) = \frac{\prod_{k=1}^K \Gamma(x_k)}{\Gamma(\sum_{k=1}^K x_k)}$  and  $\Gamma(\cdot)$  is the gamma function. The terms in  $\mathbb{E}_\gamma[\log \gamma]$ ,  $\mathbb{E}_\eta[\log \eta]$ ,  $\mathbb{E}_\pi[\log \pi]$  and  $\log(2\pi)$  do simplify in (7) after the VBEM update step. This leads to

$$\begin{aligned}
\mathcal{L}_K(q; \xi) = & \frac{1}{2} \sum_{i \neq j}^n \left\{ (Y_{ij} - \frac{1}{2})(\mathbb{E}_{Z_i, Z_j, \alpha}[Z_i^\top \alpha Z_j] + x_{ij}^\top \mathbb{E}_\beta[\beta]) + \log g(\xi_{ij}) - \frac{\xi_{ij}}{2} \right. \\
& \left. - \lambda(\xi_{ij}) (\mathbb{E}_{Z_i, Z_j, \alpha}[(Z_i^\top \alpha Z_j)^2] + 2\mathbb{E}_{Z_i, Z_j, \alpha}[Z_i^\top \alpha Z_j] x_{ij}^\top \mathbb{E}_\beta[\beta] + \mathbb{E}_\beta[(x_{ij}^\top \beta)^2] - \xi_{ij}^2) \right\} \\
& - \log C(e) - \frac{a_n}{2b_n} \sum_{k \leq l}^K \mathbb{E}_{\alpha_{kl}}[\alpha_{kl}^2] - \frac{c_n}{2d_n} \text{Tr}(S_\beta + m_\beta m_\beta^\top) \\
& - \log \Gamma(a_0) + a_0 \log b_0 - b_0 \frac{a_n}{b_n} - \log \Gamma(c_0) + c_0 \log d_0 - d_0 \frac{c_n}{d_n} \\
& - \sum_{i=1}^n \sum_{k=1}^K \tau_{ik} \log \tau_{ik} + \log C(e^n) + \frac{1}{2} \sum_{k \leq l}^K \log(\sigma_\alpha^2)_{kl} + \frac{1}{2} \sum_{k \leq l}^K (\sigma_\alpha^2)^{-1}_{kl} \mathbb{E}_{\alpha_{kl}}[\alpha_{kl}^2] \\
& - \frac{1}{2} \sum_{k \leq l}^K (\sigma_\alpha^2)^{-1}_{kl} (m_\alpha)_{kl}^2 + \frac{1}{2} \log |S_\beta| + \frac{1}{2} \text{Tr}(S_\beta^{-1}(S_\beta + m_\beta(m_\beta)^\top)) \\
& - \frac{1}{2} m_\beta^\top S_\beta^{-1} m_\beta + \log \Gamma(a_n) - a_n \log b_n + b_n \frac{a_n}{b_n} + \log \Gamma(c_n) \\
& - c_n \log d_n + d_n \frac{c_n}{d_n}.
\end{aligned}$$

Moreover, using (5), note that

$$\begin{aligned}
\frac{1}{2} \sum_{i \neq j}^n (Y_{ij} - \frac{1}{2}) \mathbb{E}_{Z_i, Z_j, \alpha}[Z_i^\top \alpha Z_j] &= \sum_{k=1}^K \mathbb{E}_{\alpha_{kk}}[\alpha_{kk}] \frac{1}{2} \sum_{i \neq j}^n (Y_{ij} - \frac{1}{2}) \tau_{ik} \tau_{jk} \\
&+ \sum_{k < l}^K \mathbb{E}_{\alpha_{kl}}[\alpha_{kl}] \sum_{i \neq j}^n (Y_{ij} - \frac{1}{2}) \tau_{ik} \tau_{jl}, \\
\frac{1}{2} \sum_{i \neq j}^n 2\lambda(\xi_{ij}) \mathbb{E}_{Z_i, Z_j, \alpha}[Z_i^\top \alpha Z_j] x_{ij}^\top \mathbb{E}_\beta[\beta] &= \sum_{k=1}^K \mathbb{E}_{\alpha_{kk}}[\alpha_{kk}] \sum_{i \neq j}^n \lambda(\xi_{ij}) x_{ij}^\top \mathbb{E}_\beta[\beta] \tau_{ik} \tau_{jk} \\
&+ \sum_{k < l}^K \mathbb{E}_{\alpha_{kl}}[\alpha_{kl}] 2 \sum_{i \neq j}^n \lambda(\xi_{ij}) x_{ij}^\top \mathbb{E}_\beta[\beta] \tau_{ik} \tau_{jl}.
\end{aligned}$$

Using (3) and (5),

$$\begin{aligned} \frac{1}{2} \sum_{i \neq j}^n \lambda(\xi_{ij}) \mathbb{E}_{Z_i, Z_j, \alpha} [(Z_i^\top \alpha Z_j)^2] &= \sum_{k=1}^K \mathbb{E}_{\alpha_{kk}} [\alpha_{kk}^2] \frac{1}{2} \sum_{i \neq j}^n \lambda(\xi_{ij}) \tau_{ik} \tau_{jk} \\ &\quad + \sum_{k < l}^K \mathbb{E}_{\alpha_{kl}} [\alpha_{kl}^2] \sum_{i \neq j}^n \lambda(\xi_{ij}) \tau_{ik} \tau_{jl} \end{aligned}$$

Finally

$$\begin{aligned} \mathbb{E}_\beta [(x_{ij}^\top \beta)^2] &= \mathbb{E}_\beta [x_{ij}^\top \beta x_{ij}^\top \beta] \\ &= \mathbb{E}_\beta [x_{ij}^\top \beta \beta^\top x_{ij}] \\ &= \text{Tr} (x_{ij} x_{ij}^\top \mathbb{E}_\beta [\beta \beta^\top]) \\ &= \text{Tr} (x_{ij} x_{ij}^\top (S_\beta + m_\beta m_\beta^\top)) . \end{aligned}$$

Therefore

$$\begin{aligned} \mathcal{L}_K(q; \xi) &= \frac{1}{2} \sum_{i \neq j}^n \left\{ \log g(\xi_{ij}) - \frac{\xi_{ij}}{2} + \lambda(\xi_{ij}) \xi_{ij}^2 \right\} + \log \frac{C(e^n)}{C(e)} + \log \frac{\Gamma(a_n)}{\Gamma(a_0)} + \log \frac{\Gamma(c_n)}{\Gamma(c_0)} \\ &\quad + a_0 \log b_0 + a_n (1 - \frac{b_0}{b_n} - \log b_n) + c_0 \log d_0 + c_n (1 - \frac{d_0}{d_n} - \log d_n) \\ &\quad + \frac{1}{2} \sum_{k \leq l}^K \log(\sigma_\alpha^2)_{kl} + \frac{1}{2} \log |S_\beta| - \sum_{i=1}^n \sum_{k=1}^K \tau_{ik} \log \tau_{ik} - \frac{1}{2} \sum_{k \leq l}^K (\sigma_\alpha^2)_{kl}^{-1} (m_\alpha)_{kl}^2 - \frac{1}{2} m_\beta^\top S_\beta^{-1} m_\beta \\ &\quad + \sum_{k=1}^K (m_\alpha)_{kk} \sum_{i \neq j}^n \left( \frac{1}{2} (Y_{ij} - \frac{1}{2}) - \lambda(\xi_{ij}) x_{ij}^\top m_\beta \right) \tau_{ik} \tau_{jk} \\ &\quad + \sum_{k < l}^K (m_\alpha)_{kl} \sum_{i \neq j}^n \left( (Y_{ij} - \frac{1}{2}) - 2\lambda(\xi_{ij}) x_{ij}^\top m_\beta \right) \tau_{ik} \tau_{jl} \\ &\quad - \sum_{k=1}^K \mathbb{E}_{\alpha_{kk}} [\alpha_{kk}^2] \frac{1}{2} \left( \frac{a_n}{b_n} - (\sigma_\alpha^2)_{kk}^{-1} + \sum_{i \neq j}^n \lambda(\xi_{ij}) \tau_{ik} \tau_{jk} \right) \\ &\quad - \sum_{k < l}^K \mathbb{E}_{\alpha_{kl}} [\alpha_{kl}^2] \frac{1}{2} \left( \frac{a_n}{b_n} - (\sigma_\alpha^2)_{kl}^{-1} + 2 \sum_{i \neq j}^n \lambda(\xi_{ij}) \tau_{ik} \tau_{jl} \right) \\ &\quad + \frac{1}{2} m_\beta^\top \sum_{i \neq j}^n (Y_{ij} - \frac{1}{2}) x_{ij} \\ &\quad - \frac{1}{2} \text{Tr} \left( \left( 2 \sum_{i \neq j}^n \lambda(\xi_{ij}) x_{ij} x_{ij}^\top + \frac{c_n}{d_n} I_d - S_\beta^{-1} \right) (S_\beta + m_\beta m_\beta^\top) \right) . \end{aligned}$$

Finally, since the terms at the fourth and fifth line correspond exactly to  $\sum_{k \leq l}^K (m_\alpha)_{kl} (\sigma_\alpha^2)_{kl}^{-1} (m_\alpha)_{kl}$ , and after the VBEM update step

$$\begin{aligned} \mathcal{L}_K(q; \xi) = & \frac{1}{2} \sum_{i \neq j}^n \left\{ \log g(\xi_{ij}) - \frac{\xi_{ij}}{2} + \lambda(\xi_{ij}) \xi_{ij}^2 \right\} + \log \frac{C(e^n)}{C(e)} + \log \frac{\Gamma(a_n)}{\Gamma(a_0)} + \log \frac{\Gamma(c_n)}{\Gamma(c_0)} \\ & + a_0 \log b_0 + a_n \left(1 - \frac{b_0}{b_n} - \log b_n\right) + c_0 \log d_0 + c_n \left(1 - \frac{d_0}{d_n} - \log d_n\right) \\ & + \frac{1}{2} \sum_{k \leq l}^K \log(\sigma_\alpha^2)_{kl} + \frac{1}{2} \log |S_\beta| - \sum_{i=1}^n \sum_{k=1}^K \tau_{ik} \log \tau_{ik} + \frac{1}{2} \sum_{k \leq l}^K (\sigma_\alpha^2)_{kl}^{-1} (m_\alpha)_{kl}^2 - \frac{1}{2} m_\beta^\top S_\beta^{-1} m_\beta \\ & + \frac{1}{2} m_\beta^\top \sum_{i \neq j}^n \left(Y_{ij} - \frac{1}{2}\right) x_{ij}. \end{aligned}$$

## References

- [1] T.S. Jaakkola and M.I. Jordan. Bayesian parameter estimation via variational methods. *Statistics and Computing*, 10:25–37, 2000.
