# Supplementary material for: Goodness of fit of logistic models for random graphs
Source: arXiv:1508.00286 ancillary file (2017-01-06)
Supplement: Supplementary file 2 [file directed.pdf]

# Supplementary files of “Goodness of fit of logistic models for random graphs” : the directed case

Pierre Latouche

Laboratoire SAMM, EA 4543, Université Paris 1 Panthéon-Sorbonne, France  
and

Stéphane Robin

AgroParisTech, UMR 518, MIA, Paris, France

INRA, UMR 518, MIA, Paris, France

and

Sarah Ouadah

AgroParisTech, UMR 518, MIA, Paris, France

INRA, UMR 518, MIA, Paris, France

November 23, 2015

# 1 Model

## Notations.

- $n$  nodes;
- $x_{ij}$  = vector (dimension  $d$ ) of covariates for edge  $(i, j)$ ;
- $Z_i$  = (latent) class of node  $i$ ;
- $Y_{ij}$  = edge between nodes  $i$  and  $j$

## Priors.

- (Proportions)  $\pi \sim \mathcal{D}(e)$ , where  $e$  is a vector with  $K$  components such that  $e_k = e_0, \forall k \in \{1, \dots, K\}$ ;
- (Group specific constants)  $\alpha \in \mathcal{M}_{K,K}(\mathbb{R})$ . In the following, we consider the  $\text{vec}$  operator which stacks the column of a matrix into a vector. Thus, if  $A$  is the  $2 \times 2$  matrix

$$A = \begin{pmatrix} A_{11} & A_{12} \\ A_{21} & A_{22} \end{pmatrix},$$

then

$$A^{\text{vec}} = \begin{pmatrix} A_{11} \\ A_{21} \\ A_{12} \\ A_{22} \end{pmatrix}.$$

For the group specific parameter matrix  $\alpha$ , we consider the prior distribution

$$p(\alpha^{\text{vec}}|\gamma) = \mathcal{N}(\alpha^{\text{vec}}; 0, \frac{I_{K^2}}{\gamma})$$

where  $I_{K^2}$  denotes the  $K^2 \times K^2$  identity matrix and  $\gamma$  is a parameter controlling the inverse variance;

- (Regression coefficients)  $\beta \in R^d$ . Again, we consider a Gaussian prior distribution

$$p(\beta|\eta) = \mathcal{N}(\beta; 0, \frac{I_d}{\eta})$$

with  $I_d$  the  $d \times d$  identity matrix;

- $\gamma \in \mathbb{R}^+$ . We consider a Gamma distribution  $p(\gamma) = \text{Gam}(\gamma; a_0, b_0)$ ;
- $\eta \in \mathbb{R}^+$ . We consider a Gamma distribution  $p(\eta) = \text{Gam}(\eta; c_0, d_0)$ .

**Model.**

- $(Z_i)$  iid  $|\pi, Z_i \sim \mathcal{M}(1; \pi)$ ;
- $(Y_{ij})$  independent  $|Z_i, Z_j, \alpha, \beta$

$$Y_{ij}|x_{ij}, Z_i, Z_j, \alpha, \beta \sim \mathcal{B}(g(Z_i^\top \alpha Z_j + x_{ij}^\top \beta)).$$

## 2 Inference

### 2.1 Variational approximations

We aim at considering the integrated observed data log-likelihood, also called marginal log-likelihood

$$\log p(Y|K) = \log \left\{ \sum_Z \int p(Y|X, Z, \alpha, \beta) p(Z|\pi) p(\alpha|\gamma) p(\beta|\eta) p(\pi) p(\gamma) p(\eta) d\pi d\alpha d\beta d\gamma d\eta \right\}. \quad (1)$$

Unfortunately neither (1) nor the posterior distribution  $p(Z, \pi, \alpha, \beta, \gamma, \eta|X)$  are tractable and therefore we propose to rely on variational approximations for inference purposes. Let us first consider the global variational decomposition

$$\log p(Y|K) = \mathcal{L}(q) + \text{KL}(q(\cdot)||p(\cdot|X)).$$

Maximizing the functional  $\mathcal{L}(\cdot)$ , which is a lower bound of  $\log p(Y|K)$ , with respect to the distribution  $q(\cdot)$ , is equivalent to minimizing the Kullback-Leibler divergence between  $q(\cdot)$  and the unknown posterior distribution  $p(\cdot|X)$ .  $\mathcal{L}(\cdot)$  is given by

$$\mathcal{L}(q) = \sum_Z \int q(Z, \pi, \alpha, \beta, \gamma, \eta) \log \frac{p(X, Z, \pi, \alpha, \beta, \gamma, \eta)}{q(Z, \pi, \alpha, \beta, \gamma, \eta)} d\pi d\alpha d\beta d\gamma d\eta.$$

In order to maximize the lower bound, we assume that the distribution can be factorized

$$q(Z, \pi, \alpha, \beta, \gamma, \eta) = q(\pi)q(\alpha)q(\beta)q(\gamma)q(\eta) \prod_{i=1}^n q(Z_i).$$

Unfortunately,  $\mathcal{L}(\cdot)$  is still intractable due to the logistic function in  $p(Y|X, Z, \alpha, \beta)$ . Following the work of [1], a tractable lower bound is derived

$$\mathcal{L}(q; \xi) = \sum_Z \int q(Z, \pi, \alpha, \beta, \gamma, \eta) \log \frac{h(Z, \alpha, \beta, \xi)p(Z, \pi, \alpha, \beta, \gamma, \eta)}{q(Z, \pi, \alpha, \beta, \gamma, \eta)} d\pi d\alpha d\beta d\gamma d\eta,$$

where

$$\log h(Z, \alpha, \beta, \xi) = \sum_{i \neq j}^n \left\{ (Y_{ij} - \frac{1}{2})(Z_i^\top \alpha Z_j + x_{ij}^\top \beta) + \log g(\xi_{ij}) - \frac{\xi_{ij}}{2} - \lambda(\xi_{ij}) \left( (Z_i^\top \alpha Z_j + x_{ij}^\top \beta)^2 - \xi_{ij}^2 \right) \right\}$$

with  $\xi_{ij} \in \mathbb{R}^+$  and  $\lambda(\xi_{ij}) = (g(\xi_{ij}) - 1/2) / (2\xi_{ij})$ . Please note that

$$\log(Y|K) \geq \mathcal{L}(q) \geq \mathcal{L}(q; \xi).$$

## 2.2 VBEM

In the following, we derive a variational Bayes expectation maximization (VBEM) algorithm maximizing  $\mathcal{L}(q; \xi)$ .

### 2.2.1 $q(\pi)$

$$\begin{aligned} \log q(\pi) &= \mathbb{E}_Z [\log p(Z|\pi) + \log p(\pi)] + \text{cst} \\ &= \sum_{i=1}^n \sum_{k=1}^K \tau_{ik} \log \pi_k + \sum_{k=1}^K (e_0 - 1) \log \pi_k + \text{cst} \\ &= \sum_{k=1}^K \left( e_0 + \sum_{i=1}^n \tau_{ik} - 1 \right) \log \pi_k + \text{cst}. \end{aligned}$$

Therefore

$$q(\pi) = \text{Dir}(\pi; e^n),$$

where  $e_k^n = e_0 + \sum_{i=1}^n \tau_{ik}, \forall k \in \{1, \dots, K\}$ .

### 2.2.2 $q(\gamma)$

$$\begin{aligned} \log q(\gamma) &= \mathbb{E}_\alpha [\log p(\alpha^{\text{vec}}|\gamma) + \log p(\gamma)] + \text{cst} \\ &= \mathbb{E}_\alpha \left[ \frac{K^2}{2} \log \gamma - \frac{\gamma}{2} (\alpha^{\text{vec}})^\top \alpha^{\text{vec}} \right] + (a_0 - 1) \log \gamma - b_0 \gamma + \text{cst} \\ &= (a_0 + \frac{K^2}{2} - 1) \log \gamma - \left( b_0 + \frac{1}{2} \text{Tr}(S_\alpha) + \frac{1}{2} (m_\alpha^{\text{vec}})^\top m_\alpha^{\text{vec}} \right) \gamma + \text{cst}. \end{aligned}$$

Therefore

$$q(\gamma) = \text{Gam}(\gamma; a_n, b_n),$$

where  $a_n = a_0 + \frac{K^2}{2}$  and  $b_n = b_0 + \frac{1}{2}\text{Tr}(S_\alpha) + \frac{1}{2}(m_\alpha^{\text{vec}})^\top m_\alpha^{\text{vec}}$ .

### 2.2.3 $q(\eta)$

$$\log q(\eta) = \mathbb{E}_\beta [\log p(\beta|\eta) + \log p(\eta)] + \text{cst.}$$

The derivations of  $q(\eta)$  and  $q(\gamma)$  are similar (see Section 2.2.2).

$$q(\eta) = \text{Gam}(\eta; c_n, d_n),$$

where  $c_n = c_0 + \frac{d}{2}$  and  $d_n = d_0 + \frac{1}{2}\text{Tr}(S_\beta) + \frac{1}{2}m_\beta^\top m_\beta$ .

### 2.2.4 $q(Z_i)$

$$\begin{aligned} \log q(Z_i) &= \mathbb{E}_{Z^{\setminus i}, \alpha, \beta, \pi} [\log h(Z, \alpha, \beta, \xi) + \log p(Z|\pi)] + \text{cst} \\ &= \mathbb{E}_{Z^{\setminus i}, \alpha, \beta, \pi} \left[ \sum_{i \neq j}^n \left\{ (Y_{ij} - \frac{1}{2}) Z_i^\top \alpha Z_j - \lambda(\xi_{ij}) ((Z_i^\top \alpha Z_j)^2 + 2Z_i^\top \alpha Z_i x_{ij}^\top \beta) \right\} \right. \\ &\quad \left. + \sum_{k=1}^n Z_{ik} \log \pi_k \right] + \text{cst.} \end{aligned}$$

Note that

$$\begin{aligned} \mathbb{E}_{Z_j, \alpha} [Z_i^\top \alpha Z_j] &= \mathbb{E}_{Z_j, \alpha} \left[ \sum_{k,l}^K Z_{ik} \alpha_{kl} Z_{jl} \right] \\ &= \sum_{k=1}^K Z_{ik} \left\{ \sum_{l=1}^K (m_\alpha)_{kl} \tau_{jl} \right\}. \end{aligned}$$

Furthermore

$$\begin{aligned} \mathbb{E}_{Z_j, \alpha} [(Z_i^\top \alpha Z_j)^2] &= \mathbb{E}_{Z_j, \alpha} \left[ \left( \sum_{k,l}^K Z_{ik} \alpha_{kl} Z_{jl} \right)^2 \right] \\ &= \mathbb{E}_{Z_j, \alpha} \left[ \sum_{k,k',l,l'}^K Z_{ik} Z_{ik'} \alpha_{kl} \alpha_{k'l'} Z_{jl} Z_{jl'} \right]. \end{aligned} \tag{2}$$

Because all vectors  $Z_i$  are sampled from a multinomial distribution with parameters  $(1, \pi)$ , all terms  $Z_{ik} Z_{ik'} = 0$  for  $k \neq k'$  and  $Z_{ik}^2 = Z_{ik}$  in (2). Therefore

$$(Z_i^\top \alpha Z_j)^2 = \sum_{k,l}^K Z_{ik} \alpha_{kl}^2 Z_{jl}. \tag{3}$$

This leads to

$$\mathbb{E}_{Z_j, \alpha}[(Z_i^\top \alpha Z_j)^2] = \sum_{k=1}^K Z_{ik} \left\{ \sum_{l=1}^K \mathbb{E}_{\alpha_{kl}}[\alpha_{kl}^2] \tau_{jl} \right\}.$$

Finally

$$\begin{aligned} \log q(Z_i) &= \sum_{k=1}^K Z_{ik} \left\{ \sum_{l=1}^K (m_\alpha)_{kl} \sum_{j \neq i}^n \left( (Y_{ij} - \frac{1}{2}) - 2\lambda(\xi_{ij}) x_{ij}^\top m_\beta \right) \tau_{jl} - \sum_{l=1}^K \mathbb{E}_{\alpha_{kl}}[\alpha_{kl}^2] \sum_{j \neq i}^n \lambda(\xi_{ij}) \tau_{jl} \right. \\ &+ \sum_{l=1}^K (m_\alpha)_{lk} \sum_{j \neq i}^n \left( (Y_{ji} - \frac{1}{2}) - 2\lambda(\xi_{ji}) x_{ji}^\top m_\beta \right) \tau_{jl} - \sum_{l=1}^K \mathbb{E}_{\alpha_{lk}}[\alpha_{lk}^2] \sum_{j \neq i}^n \lambda(\xi_{ji}) \tau_{jl} \\ &\left. + \psi(e_k^n) - \psi\left(\sum_{l=1}^K e_l^n\right) \right\} + \text{cst.} \end{aligned}$$

Therefore

$$q(Z_i) = \mathcal{M}(Z_i; 1, \tau_i),$$

where  $\sum_{k=1}^K \tau_{ik} = 1$  and

$$\begin{aligned} \tau_{ik} &\propto \exp \left\{ \sum_{l=1}^K (m_\alpha)_{kl} \sum_{j \neq i}^n \left( (Y_{ij} - \frac{1}{2}) - 2\lambda(\xi_{ij}) x_{ij}^\top m_\beta \right) \tau_{jl} - \sum_{l=1}^K \mathbb{E}_{\alpha_{kl}}[\alpha_{kl}^2] \sum_{j \neq i}^n \lambda(\xi_{ij}) \tau_{jl} \right. \\ &+ \sum_{l=1}^K (m_\alpha)_{lk} \sum_{j \neq i}^n \left( (Y_{ji} - \frac{1}{2}) - 2\lambda(\xi_{ji}) x_{ji}^\top m_\beta \right) \tau_{jl} - \sum_{l=1}^K \mathbb{E}_{\alpha_{lk}}[\alpha_{lk}^2] \sum_{j \neq i}^n \lambda(\xi_{ji}) \tau_{jl} \\ &\left. + \psi(e_k^n) - \psi\left(\sum_{l=1}^K e_l^n\right) \right\}. \end{aligned}$$

### 2.2.5 $q(\alpha^{\text{vec}})$

$$\begin{aligned} \log q(\alpha^{\text{vec}}) &= \mathbb{E}_{Z, \beta, \gamma} [\log h(Z, \alpha, \beta, \xi) + \log p(\alpha^{\text{vec}} | \gamma)] + \text{cst} \\ &= \mathbb{E}_{Z, \beta, \gamma} \left[ \sum_{i \neq j}^n \left\{ (Y_{ij} - \frac{1}{2}) Z_i^\top \alpha Z_j - \lambda(\xi_{ij}) \left( (Z_i^\top \alpha Z_j)^2 + 2Z_i^\top \alpha Z_j x_{ij}^\top \beta \right) \right\} \right. \\ &\quad \left. - \frac{\gamma}{2} (\alpha^{\text{vec}})^\top \alpha^{\text{vec}} \right] + \text{cst.} \end{aligned}$$

First note that

$$\begin{aligned} \mathbb{E}_{Z_i, Z_j} [Z_i^\top \alpha Z_j] &= \tau_i^\top \alpha \tau_j \\ &= (\alpha^{\text{vec}})^\top (\tau_j \otimes \tau_i), \end{aligned}$$

where  $\otimes$  denotes the Kronecker product. Moreover

$$\mathbb{E}_{Z_i, Z_j} [(Z_i^\top \alpha Z_j)^2] = \mathbb{E}_{Z_i, Z_j} \left[ \sum_{k,l}^K Z_{ik} \alpha_{kl}^2 Z_{jl} \right],$$

following (3). Therefore

$$\begin{aligned} \mathbb{E}_{Z_i, Z_j} [(Z_i^\top \alpha Z_j)^2] &= \sum_{k,l}^K \tau_{ik} \alpha_{kl}^2 \tau_{jl} \\ &= (\alpha^{\text{vec}})^\top E_{ij} \alpha^{\text{vec}}, \end{aligned}$$

where

$$E_{ij} = \begin{pmatrix} [E_{ij}^1] & 0 & \dots & \dots & 0 \\ 0 & [E_{ij}^2] & 0 & \dots & \vdots \\ \vdots & 0 & [\cdot \cdot] & 0 & \vdots \\ \vdots & \vdots & 0 & [\cdot \cdot] & 0 \\ 0 & \dots & \dots & 0 & [E_{ij}^K] \end{pmatrix},$$

and  $(E_{ij}^l)_{kk'} = 0$  for  $k \neq k'$  and  $(E_{ij}^l)_{kk} = \tau_{ik} \tau_{jl}$  for all  $k$  in  $\{1, \dots, K\}$ . Thus

$$\begin{aligned} \log q(\alpha^{\text{vec}}) &= (\alpha^{\text{vec}})^\top \sum_{i \neq j}^n \left( (Y_{ij} - \frac{1}{2}) - 2\lambda(\xi_{ij}) x_{ij}^\top m_\beta \right) (\tau_j \otimes \tau_i) \\ &\quad - \frac{1}{2} (\alpha^{\text{vec}})^\top \left( \frac{a_n}{b_n} I_{K^2} + 2 \sum_{i \neq j}^n \lambda(\xi_{ij}) E_{ij} \right) \alpha^{\text{vec}} + \text{cst}. \end{aligned}$$

Finally

$$q(\alpha^{\text{vec}}) = \mathcal{N}(\alpha^{\text{vec}}; m_\alpha^{\text{vec}}, S_\alpha),$$

where

$$S_\alpha^{-1} = \frac{a_n}{b_n} I_{K^2} + 2 \sum_{i \neq j}^n \lambda(\xi_{ij}) E_{ij},$$

and

$$m_\alpha^{\text{vec}} = S_\alpha \sum_{i \neq j}^n \left( Y_{ij} - \frac{1}{2} - 2\lambda(\xi_{ij}) x_{ij}^\top m_\beta \right) (\tau_j \otimes \tau_i).$$

Please note that  $S_\alpha^{-1}$  is a diagonal matrix and so is  $S_\alpha$ . Thus,  $q(\alpha^{\text{vec}})$  is in fact a product of unidimensional distributions  $q(\alpha_j^{\text{vec}})$ . However, to limit the use of sums in the rest of the paper, and to facilitate the comparison of  $q(\alpha^{\text{vec}})$  and  $q(\beta)$ , we keep these matrix notations.

### 2.2.6 $q(\beta)$

$$\begin{aligned}
\log q(\beta) &= \mathbb{E}_{Z,\alpha,\eta} [\log h(Z, \alpha, \beta, \xi) + \log p(\beta|\eta)] + \text{cst} \\
&= \mathbb{E}_{Z,\alpha,\eta} \left[ \sum_{i \neq j}^n \left\{ (Y_{ij} - 1/2)x_{ij}^\top \beta - \lambda(\xi_{ij}) \left( (x_{ij}^\top \beta)^2 + 2Z_i^\top \alpha Z_j x_{ij}^\top \beta \right) \right\} - \frac{\eta}{2} \beta^\top \beta \right] + \text{cst} \\
&= \beta^\top \left\{ \sum_{i \neq j}^n \left( Y_{ij} - \frac{1}{2} - 2\lambda(\xi_{ij}) \tau_i^\top m_\alpha \tau_j \right) x_{ij} \right\} - \frac{1}{2} \beta^\top \left\{ \frac{c_n}{d_n} I_d + 2 \sum_{i \neq j}^n \lambda(\xi_{ij}) x_{ij} x_{ij}^\top \right\} \beta + \text{cst}.
\end{aligned}$$

Therefore

$$q(\beta) = \mathcal{N}(\beta; m_\beta, S_\beta),$$

where

$$S_\beta^{-1} = \frac{c_n}{d_n} I_d + 2 \sum_{i \neq j}^n \lambda(\xi_{ij}) x_{ij} x_{ij}^\top,$$

and

$$m_\beta = S_\beta \sum_{i \neq j}^n \left( Y_{ij} - \frac{1}{2} - 2\lambda(\xi_{ij}) \tau_i^\top m_\alpha \tau_j \right) x_{ij}.$$

## 2.3 Derivation of the lower bound

$$\mathcal{L}(q; \xi) = \mathbb{E}_{Z,\pi,\alpha,\beta,\gamma,\eta} [\log h(Z, \alpha, \beta, \xi) + \log p(Z, \pi, \alpha, \beta, \gamma, \eta)] - \mathbb{E}_{Z,\pi,\alpha,\beta,\gamma,\eta} [\log q(Z, \pi, \alpha, \beta, \gamma, \eta)]$$

$$\begin{aligned}
\mathcal{L}(q; \xi) = & \sum_{i \neq j}^n \left\{ (Y_{ij} - \frac{1}{2})(\mathbb{E}_{Z_i, Z_j, \alpha}[Z_i^\top \alpha Z_j] + x_{ij}^\top \mathbb{E}_\beta[\beta]) + \log g(\xi_{ij}) - \frac{\xi_{ij}}{2} \right. \\
& \left. - \lambda(\xi_{ij}) (\mathbb{E}_{Z_i, Z_j, \alpha}[(Z_i^\top \alpha Z_j)^2] + 2\mathbb{E}_{Z_i, Z_j, \alpha}[Z_i^\top \alpha Z_j] x_{ij}^\top \mathbb{E}_\beta[\beta] + \mathbb{E}_\beta[(x_{ij}^\top \beta)^2] - \xi_{ij}^2) \right\} \\
& + \sum_{i=1}^n \sum_{k=1}^K \mathbb{E}_{Z_i}[Z_{ik}] \mathbb{E}_\pi[\log \pi_k] - \log C(e) + \sum_{k=1}^K (e_0 - 1) \mathbb{E}_\pi[\log \pi_k] - \frac{K^2}{2} \log(2\pi) \\
& + \frac{K^2}{2} \mathbb{E}_\gamma[\log \gamma] - \frac{\mathbb{E}_\gamma[\gamma]}{2} \mathbb{E}_\alpha[(\alpha^{\text{vec}})^\top \alpha^{\text{vec}}] - \frac{d}{2} \log(2\pi) + \frac{d}{2} \mathbb{E}_\eta[\log \eta] - \frac{\mathbb{E}_\eta[\eta]}{2} \mathbb{E}_\beta[\beta^\top \beta] \\
& - \log \Gamma(a_0) + a_0 \log b_0 + (a_0 - 1) \mathbb{E}_\gamma[\log \gamma] - b_0 \mathbb{E}_\gamma[\gamma] - \log \Gamma(c_0) \\
& + c_0 \log d_0 + (c_0 - 1) \mathbb{E}_\eta[\log \eta] - d_0 \mathbb{E}_\eta[\eta] - \sum_{i=1}^n \sum_{k=1}^K \mathbb{E}_{Z_i}[Z_{ik}] \log \tau_{ik} + \log C(e^n) \\
& - \sum_{k=1}^K (e_k^n - 1) \mathbb{E}_\pi[\log \pi_k] + \frac{K^2}{2} \log(2\pi) + \frac{1}{2} \log |S_\alpha| + \frac{1}{2} \mathbb{E}_\alpha[(\alpha^{\text{vec}})^\top S_\alpha^{-1} \alpha^{\text{vec}}] \\
& - \mathbb{E}_\alpha[\alpha^{\text{vec}}]^\top S_\alpha^{-1} m_\alpha^{\text{vec}} + \frac{1}{2} (m_\alpha^{\text{vec}})^\top S_\alpha^{-1} m_\alpha^{\text{vec}} + \frac{d}{2} \log(2\pi) + \frac{1}{2} \log |S_\beta| \\
& + \frac{1}{2} \mathbb{E}_\beta[\beta^\top S_\beta^{-1} \beta] - \mathbb{E}_\beta[\beta]^\top S_\beta^{-1} m_\beta + \frac{1}{2} m_\beta^\top S_\beta^{-1} m_\beta + \log \Gamma(a_n) - a_n \log b_n \\
& - (a_n - 1) \mathbb{E}_\gamma[\log \gamma] + b_n \mathbb{E}_\gamma[\gamma] + \log \Gamma(c_n) - c_n \log d_n - (c_n - 1) \mathbb{E}_\eta[\log \eta] \\
& + d_n \mathbb{E}_\eta[\eta], \quad (4)
\end{aligned}$$



Therefore

$$\begin{aligned}
\mathcal{L}(q; \xi) &= \sum_{i \neq j}^n \left\{ \log g(\xi_{ij}) - \frac{\xi_{ij}}{2} + \lambda(\xi_{ij})\xi_{ij}^2 \right\} + \log \frac{C(e^n)}{C(e)} + \log \frac{\Gamma(a_n)}{\Gamma(a_0)} + \log \frac{\Gamma(c_n)}{\Gamma(c_0)} \\
&\quad + a_0 \log b_0 + a_n \left(1 - \frac{b_0}{b_n} - \log b_n\right) + c_0 \log d_0 + c_n \left(1 - \frac{d_0}{d_n} - \log d_n\right) \\
&\quad + \frac{1}{2} \log |S_\alpha| + \frac{1}{2} \log |S_\beta| - \sum_{i=1}^n \sum_{k=1}^K \tau_{ik} \log \tau_{ik} - \frac{1}{2} (m_\alpha^{\text{vec}})^\top S_\alpha^{-1} m_\alpha^{\text{vec}} - \frac{1}{2} m_\beta^\top S_\beta^{-1} m_\beta \\
&\quad + (m_\alpha^{\text{vec}})^\top \sum_{i \neq j}^n \left( Y_{ij} - \frac{1}{2} - 2\lambda(\xi_{ij})x_{ij}^\top m_\beta \right) (\tau_j \otimes \tau_i) \\
&\quad - \frac{1}{2} \text{Tr} \left( \left( 2 \sum_{i \neq j}^n \lambda(\xi_{ij}) E_{ij} + \frac{a_n}{b_n} I_{K^2} - S_\alpha^{-1} \right) (S_\alpha + m_\alpha^{\text{vec}} (m_\alpha^{\text{vec}})^\top) \right) \\
&\quad \quad \quad + m_\beta^\top \sum_{i \neq j}^n \left( Y_{ij} - \frac{1}{2} \right) x_{ij} \\
&\quad - \frac{1}{2} \text{Tr} \left( \left( 2 \sum_{i \neq j}^n \lambda(\xi_{ij}) x_{ij} x_{ij}^\top + \frac{c_n}{d_n} I_d - S_\beta^{-1} \right) (S_\beta + m_\beta m_\beta^\top) \right).
\end{aligned}$$

Finally, since the term at the fourth line is exactly  $(m_\alpha^{\text{vec}})^\top S_\alpha^{-1} m_\alpha$ , and after the VBEM update step

$$\begin{aligned}
\mathcal{L}(q; \xi) &= \sum_{i \neq j}^n \left\{ \log g(\xi_{ij}) - \frac{\xi_{ij}}{2} + \lambda(\xi_{ij})\xi_{ij}^2 \right\} + \log \frac{C(e^n)}{C(e)} + \log \frac{\Gamma(a_n)}{\Gamma(a_0)} + \log \frac{\Gamma(c_n)}{\Gamma(c_0)} \\
&\quad + a_0 \log b_0 + a_n \left(1 - \frac{b_0}{b_n} - \log b_n\right) + c_0 \log d_0 + c_n \left(1 - \frac{d_0}{d_n} - \log d_n\right) \\
&\quad + \frac{1}{2} \log |S_\alpha| + \frac{1}{2} \log |S_\beta| - \sum_{i=1}^n \sum_{k=1}^K \tau_{ik} \log \tau_{ik} + \frac{1}{2} (m_\alpha^{\text{vec}})^\top S_\alpha^{-1} m_\alpha^{\text{vec}} - \frac{1}{2} m_\beta^\top S_\beta^{-1} m_\beta \\
&\quad \quad \quad + m_\beta^\top \sum_{i \neq j}^n \left( Y_{ij} - \frac{1}{2} \right) x_{ij}.
\end{aligned}$$

## 2.4 Local variational optimization

Keeping only the terms that do depend on  $\xi_{ij}$  in (4), the lower bound is given by

$$\begin{aligned}
\mathcal{L}(q; \xi) &= \sum_{i \neq j}^n \left\{ \log g(\xi_{ij}) - \frac{\xi_{ij}}{2} - \lambda(\xi_{ij}) \left( \text{Tr}(E_{ij}(S_\alpha + m_\alpha^{\text{vec}} (m_\alpha^{\text{vec}})^\top)) + 2\tau_i^\top m_\alpha \tau_j x_{ij}^\top m_\beta \right. \right. \\
&\quad \quad \quad \left. \left. + \text{Tr}(x_{ij} x_{ij}^\top (S_\beta + m_\beta m_\beta^\top)) - \xi_{ij}^2 \right) \right\} + \text{cst.}
\end{aligned}$$

The partial derivative of the lower bound with respect to  $\xi_{ij}$  is

$$\begin{aligned} \frac{\partial \mathcal{L}}{\partial \xi_{ij}}(q; \xi) = & g(-\xi_{ij}) - \frac{1}{2} - \lambda'(\xi_{ij}) \left( \text{Tr}(E_{ij}(S_\alpha + m_\alpha^{\text{vec}}(m_\alpha^{\text{vec}})^\top)) + 2\tau_i^\top m_\alpha \tau_j x_{ij}^\top m_\beta \right. \\ & \left. + \text{Tr}(x_{ij} x_{ij}^\top (S_\beta + m_\beta m_\beta^\top)) - \xi_{ij}^2 \right) + 2\lambda(\xi_{ij})\xi_{ij}, \end{aligned}$$

and

$$\begin{aligned} \frac{\partial \mathcal{L}}{\partial \xi_{ij}}(q; \xi) = & -\lambda'(\xi_{ij}) \left( \text{Tr}(E_{ij}(S_\alpha + m_\alpha^{\text{vec}}(m_\alpha^{\text{vec}})^\top)) + 2\tau_i^\top m_\alpha \tau_j x_{ij}^\top m_\beta \right. \\ & \left. + \text{Tr}(x_{ij} x_{ij}^\top (S_\beta + m_\beta m_\beta^\top)) - \xi_{ij}^2 \right). \quad (5) \end{aligned}$$

Finally,  $\lambda(\xi_{ij})$  is a strictly decreasing function for positive values of  $\xi_{ij}$ . Thus,  $\lambda'(\xi_{ij}) \neq 0$  and therefore if we set (5) to zero, we obtain

$$\xi_{ij}^2 = \text{Tr}(E_{ij}(S_\alpha + m_\alpha^{\text{vec}}(m_\alpha^{\text{vec}})^\top)) + 2\tau_i^\top m_\alpha \tau_j x_{ij}^\top m_\beta + \text{Tr}(x_{ij} x_{ij}^\top (S_\beta + m_\beta m_\beta^\top)).$$

## References

- [1] T.S. Jaakkola and M.I. Jordan. Bayesian parameter estimation via variational methods. *Statistics and Computing*, 10:25–37, 2000.
